# Supplementary material for: A study on the effects of mixed explicit and implicit communications in human-artificial-agent interactions
Source: arXiv:2409.18745 source file (2026-11-10)
Supplement: Supplementary file 1 [file supplementary.pdf]

# Supplementary Material: *A study on the effects of mixed explicit and implicit communications in human-virtual-agent interactions*

Ana Christina Almada Campos[1*] and Bruno Vilhena Adorno[2]

[1]Graduate Program in Electrical Engineering, Universidade Federal de Minas Gerais, Av. Antônio Carlos 6627, Belo Horizonte, 31270-901, MG, Brazil. ORCID: https://orcid.org/0000-0002-7800-5640.

[2]Manchester Centre for Robotics and AI, The University of Manchester, Oxford Rd, Manchester, M13 9PL, UK. ORCID: https://orcid.org/0000-0002-5080-8724.

*Corresponding author(s). E-mail(s): campos.aca@outlook.com; Contributing authors: bruno.adorno@manchester.ac.uk;

This supplementary material shows the complete results of the experiment described in the main paper to compare two communication configurations, EX and EXIM. It includes the posterior distributions of all parameters estimated, and a posterior check of model adequacy, comparing the data sample with the estimations. Section 1 shows the results for the objective measures, namely time and number of errors. The results for the subjective measures, that is, acceptance, sociability, transparency of the virtual agents, and perceived efficiency of the interaction, are shown in Section 2. For the discussions about the results, please refer to Sections 5 and 6 of the main paper.

## 1 Objective measures results

For the objective measures of time and number of errors, we use the metric model described in Section 4.2 of the main paper. We estimate the mean $\mu$, scale $\tau$, and normality parameter $\nu$ of the latent $t$ distributions of the difference in time $\Delta t = t_{\mathrm{EX}} - t_{\mathrm{EXIM}}$ and number of errors $\Delta e = e_{\mathrm{EX}} - e_{\mathrm{EXIM}}$, and calculate the effect sizes using Eq. 4 in the main paper. Also, some credible $t$ distributions were superimposed on the data of each variable to check model adequacy.

Fig. 1 shows the results for difference in time and Fig. 2 for the difference in the number of errors, with and without outliers. We show the posteriors for the normality parameter $\nu$ in log scale to ease visualization, since its distribution is very asymmetric in a linear scale. Most variation in the tails of the $t$ distribution occur for small values of $\nu$, and values greater than $\log(\nu) = 1.47$ ($\nu = 30$ in the original scale) represent distributions very close to a normal [1].

## 2 Subjective measures results

Fig. 3 shows histograms with participants' responses to each item and group for all the subjective measures, namely acceptance, sociability, transparency of the virtual agents, and perceived efficiency of the interactions.

The ordinal model used for the subjective measures is described in Section 4.3 of the main paper. We estimate the mean $\mu$, scale $\tau$, and normality parameter $\nu$ of the latent $t$ distributions, and the free thresholds $\theta_k$, with $k \in \{1, ..., K-1\}$, where

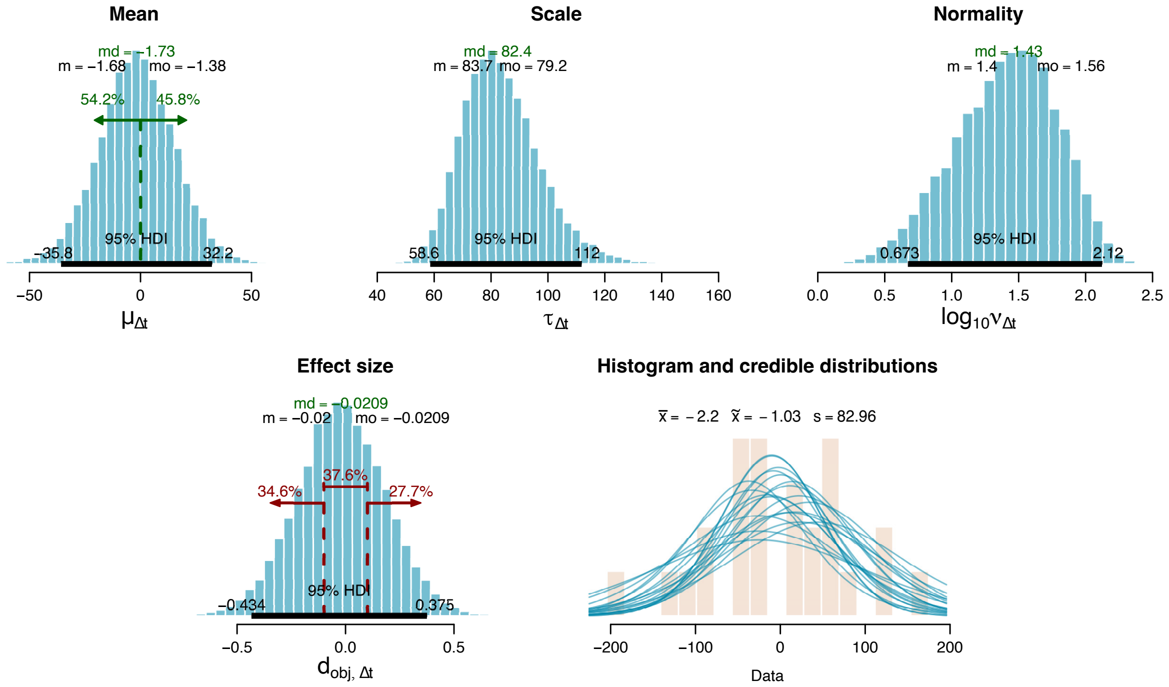


**Fig. 1** Results of the Bayesian inference of the time difference $\Delta t$ between EX and EXIM configurations, in seconds. The first row shows the posterior distributions of the mean $\mu$, scale $\tau$, and normality $\nu$ (in log scale) of the latent $t$ distribution. On the left of the second row is the distribution of the effect size $d_{\text{obj}}$ calculated with the null value $\mu_0 = 0$. Mean $(m)$, median $(md)$, mode $(mo)$, and the limits of the 95% HDI are annotated in the distributions. Dashed vertical lines indicate the null value in the distribution of the mean $\mu$ and the ROPE in the effect size distribution together with the percentages of the distribution below, between and above the values associated with the ROPE and the null value. On the right of the second row, some credible $t$ distributions are superimposed on the data to check model adequacy, and sample mean $(\bar{x})$, median $(\tilde{x})$, and standard deviation $(s)$ are shown.

$K = 5$ is the number of ordinal levels. We interpret the estimation of the mean $\mu$ considering the five ordinal levels of response (see example in Fig. 8 in Section 4.3 of the main paper). Remember that, according to the model, the ordinal response scale is a way of accessing the latent distribution, which is not limited by the response options. Thus, the estimated credible values of the mean $\mu$ of the latent distribution can be lower than 1 and higher than 5, like in some of the distributions we obtained. We also calculate the difference between the means and scales of each condition, and the effect sizes $d_{\text{sub}}$ for each variable using Eq. 5 in the main paper.

The item thresholds, which translate the latent variable into the ordinal responses, are strongly correlated, so we present their estimations together, like Kruschke [1].[1] Fig. 4 shows example posterior distributions of the thresholds of an item, represented by the blue points clouds. The spread of the clouds indicate the spread of the distributions and the dashed vertical lines indicate the estimated mean of each threshold. The example data sample contains more answers in the higher response levels so the estimations of the higher thresholds are more precise than the lower ones. The ellipses on Fig. 4 cover 95% of the clouds of thresholds $\theta_1$ (on the left) and $\theta_4$ (on the right) and the $\theta_1$ ellipse is larger than the $\theta_4$ ellipse, indicating that the $\theta_4$ posterior distribution is more compact, *i.e.*, a more precise estimation.

[1] The figures in this document containing our results were generated using the scripts provided by Kruschke and Liddell [1, 2] and adapted to our work.

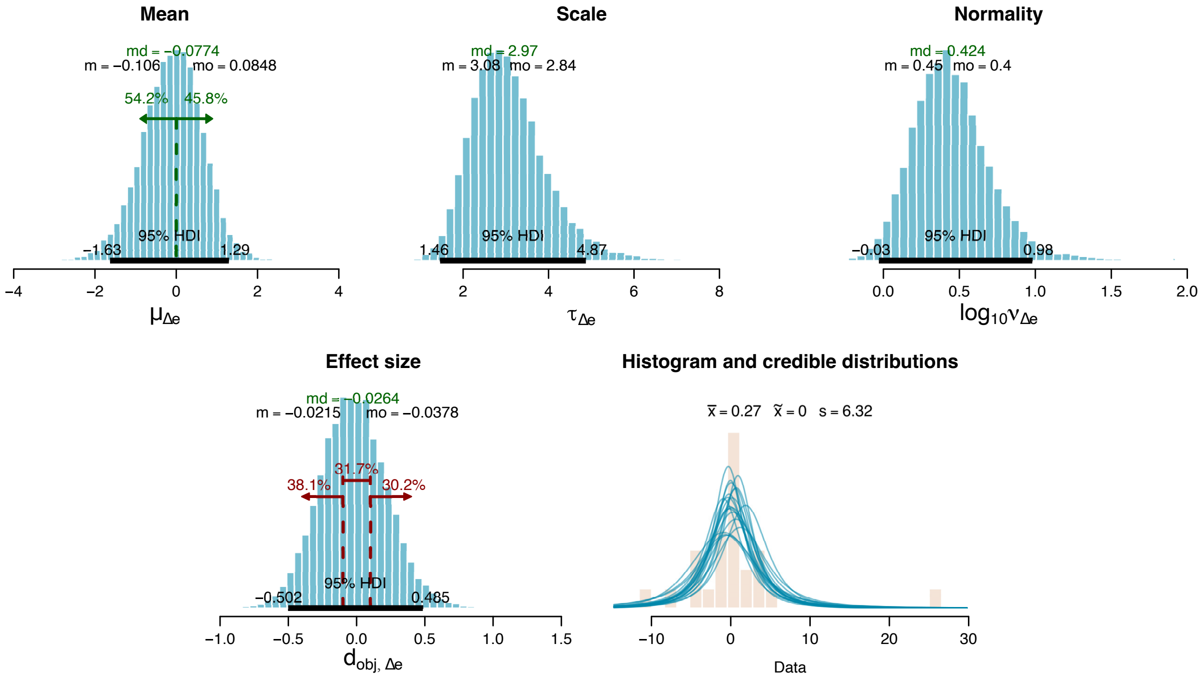


**(a)** Results for the difference in number of errors $\Delta e$.

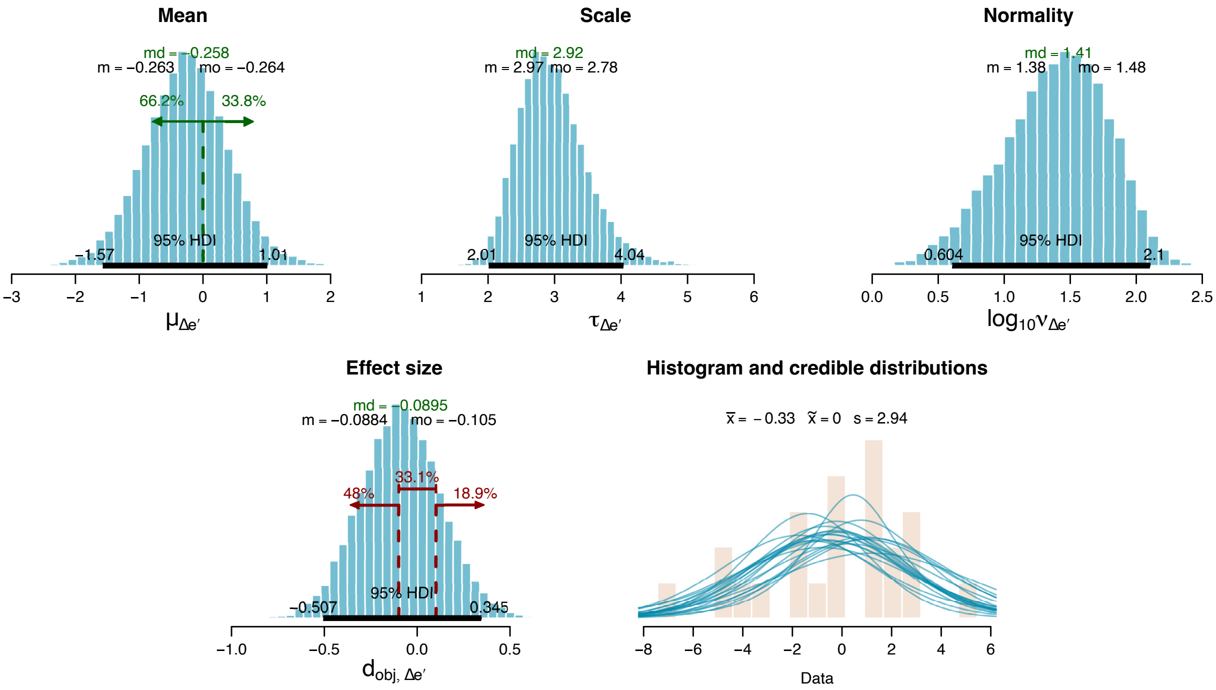


**(b)** Results for the difference in number of errors $\Delta e'$ without outliers.

**Fig. 2** Results of the Bayesian inference of the difference in the number of errors between EX and EXIM configurations, with and without outliers. In each figure, the first row shows the posterior distributions of the mean $\mu$, scale $\tau$, and normality $\nu$ (in log scale) of the latent $t$ distribution. On the left of the second row of each figure is the distribution of the effect size $d_{\text{obj}}$ calculated with the null value $\mu_0 = 0$. Mean ($m$), median ($md$), mode ($mo$), and the limits of the 95% HDI are annotated in the distributions. Dashed vertical lines indicate the null value in the distribution of the mean $\mu$ and the ROPE in the effect size distribution together with the percentages of the distribution below, between and above the values associated with the ROPE and the null value. On the right of the second row, some credible $t$ distributions are superimposed on the data to check model adequacy, and sample mean ($\bar{x}$), median ($\tilde{x}$), and standard deviation ($s$) are shown.

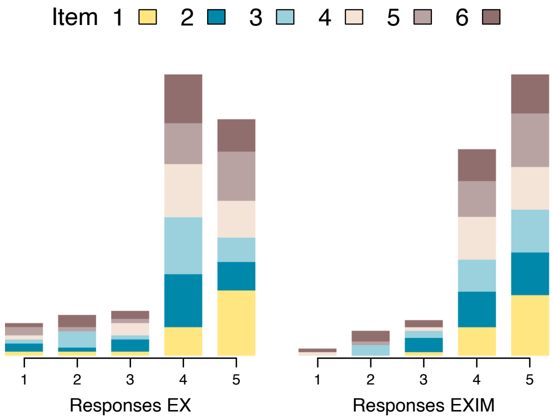


**(a)** Acceptance of the virtual agent.

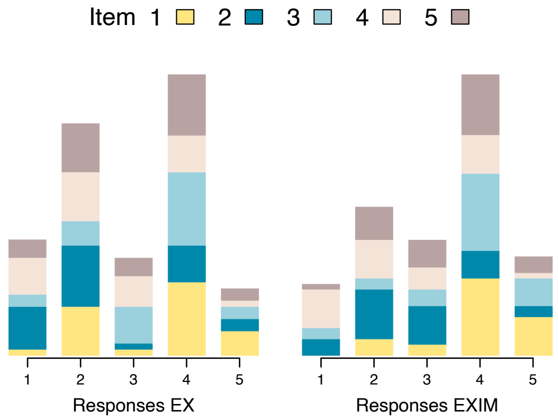


**(b)** Sociability of the virtual agent.

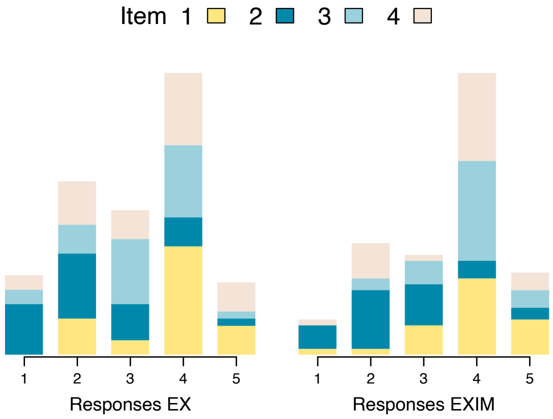


**(c)** Transparency of the virtual agent.

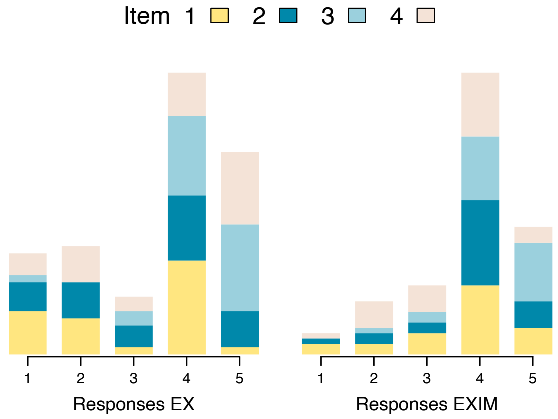


**(d)** Perceived efficiency of the interaction.

**Fig. 3** Histograms of the ordinal responses (five levels) in each item of the Likert scale for the subjective measures in EX and EXIM groups.

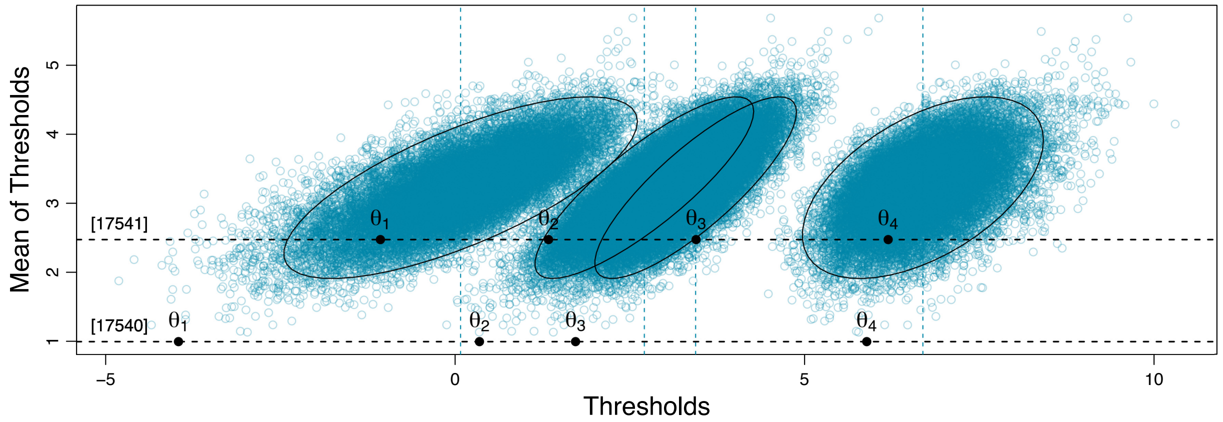


**Fig. 4** Example of posterior distributions of the thresholds $\theta_1$, $\theta_2$, $\theta_3$, and $\theta_4$ of an item.

The small blue circles in Fig. 4 represent the thresholds values in each combination of parameters in the MCMC (Markov Chain Monte Carlo) sample, and the vertical coordinate is the mean of the four thresholds in that combination. For each step of the generated MCMC sample,[2] the points are at the same height in the plot. The horizontal dashed lines are related to two subsequent steps in the MCMC sample generation, steps 17540 and 17541,[3] and the height of the lines is the mean of the thresholds (black dots) in each step. During the generation of the MCMC sample, if a higher value is chosen for a threshold, all the other item thresholds will need to adjust and tend to be higher too, to keep the probability of each ordinal response level, calculated as the cummulative probability between two consecutive thresholds in the latent distribution (see Section 4.3 in the main paper). With that, each new step tends to shift the thresholds set up and right or down and left, as we see by the subsequent steps shown in Fig. 4.

Figs. 5 and 6 show the posterior distributions for the acceptance of the virtual agents. The extreme thresholds $\theta_1^{[1]}$ and $\theta_{K-1}^{[1]}$ of the first item of each scale are always at 1.5 and 4.5, since they were fixed at these values.

For the model adequacy check, we estimate the probability of each ordinal level using the estimated parameters. Fig. 7 shows the final acceptance data histograms (with the extra answers included, as explained in the Section 4.3 and Appendix A of the main paper) superimposed with the median of the estimated probability of each level and its 95% HDI. Levels that were originally empty and for which we added an extra answer are indicated in Fig. 7 by asterisks.

Figs. 8 to 10 show the results for the sociability of the virtual agents, Figs. 11 to 13 show the results for their transparency, and Figs. 14 to 16 show the results for the perceived efficiency of the interactions.

[2] For more information about the MCMC sample generation, please refer to Chapter 7 of [1].

[3] The generated MCMC sample contains 20000 combinations of parameters.

## References


[1] Kruschke JK (2015) Doing Bayesian Data Analysis: A Tutorial with R, JAGS, and Stan. Academic Press / Elsevier, Burlington, MA

[2] Liddell TM, Kruschke JK (2018) Analyzing ordinal data with metric models: What could possibly go wrong? Journal of Experimental Social Psychology 79(August):328–348. https://doi.org/10.1016/j.jesp.2018.08.009

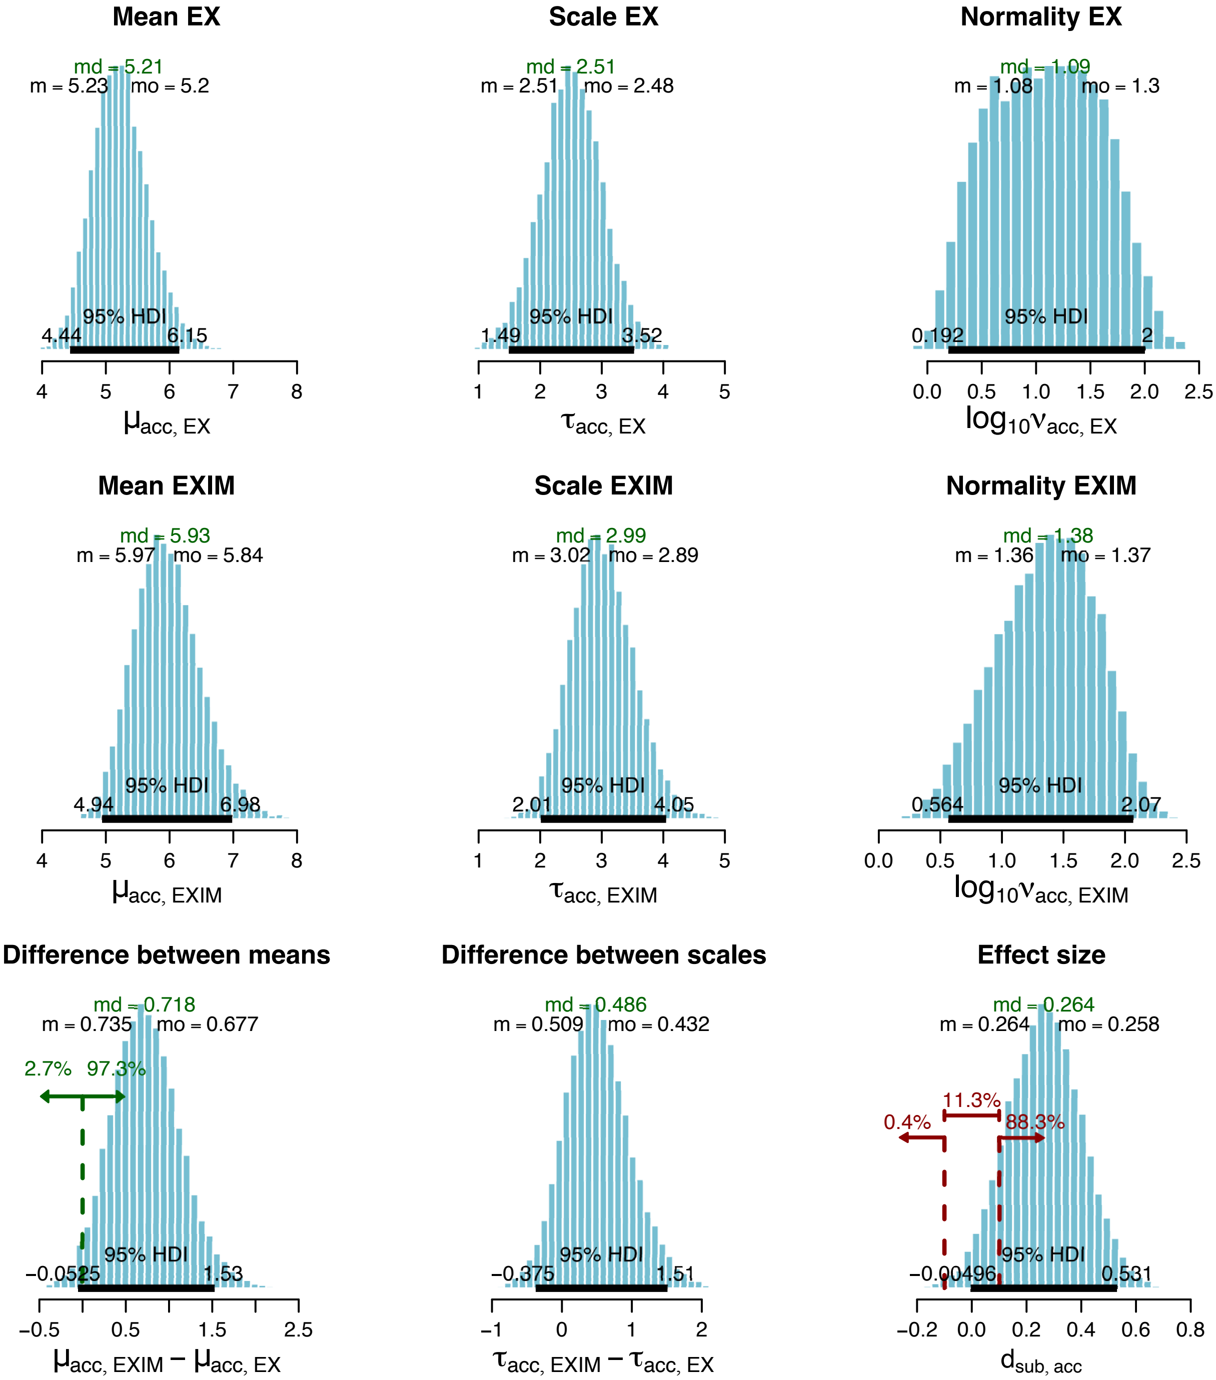


**Fig. 5** Results of the Bayesian inference of the acceptance of the virtual agents in EX and EXIM configurations. The first two rows show the posterior distributions of the mean $\mu$, scale $\tau$, and normality $\nu$ (in log scale) of the latent $t$ distribution of each group. On the left and center of the last row are the distributions of difference between the means and scales of the two groups, and on the right, the distribution of the effect size $d_{\text{sub}}$. Mean ($m$), median ($md$), mode ($mo$), and the limits of the 95% HDI are annotated in the distributions. Dashed vertical lines indicate the null value ($\mu_{\text{EXIM}} - \mu_{\text{EX}} = 0$) in the distribution of the difference between means and the ROPE in the effect size distribution together with the percentages of the distribution below, between and above the values associated with the ROPE and the null value.

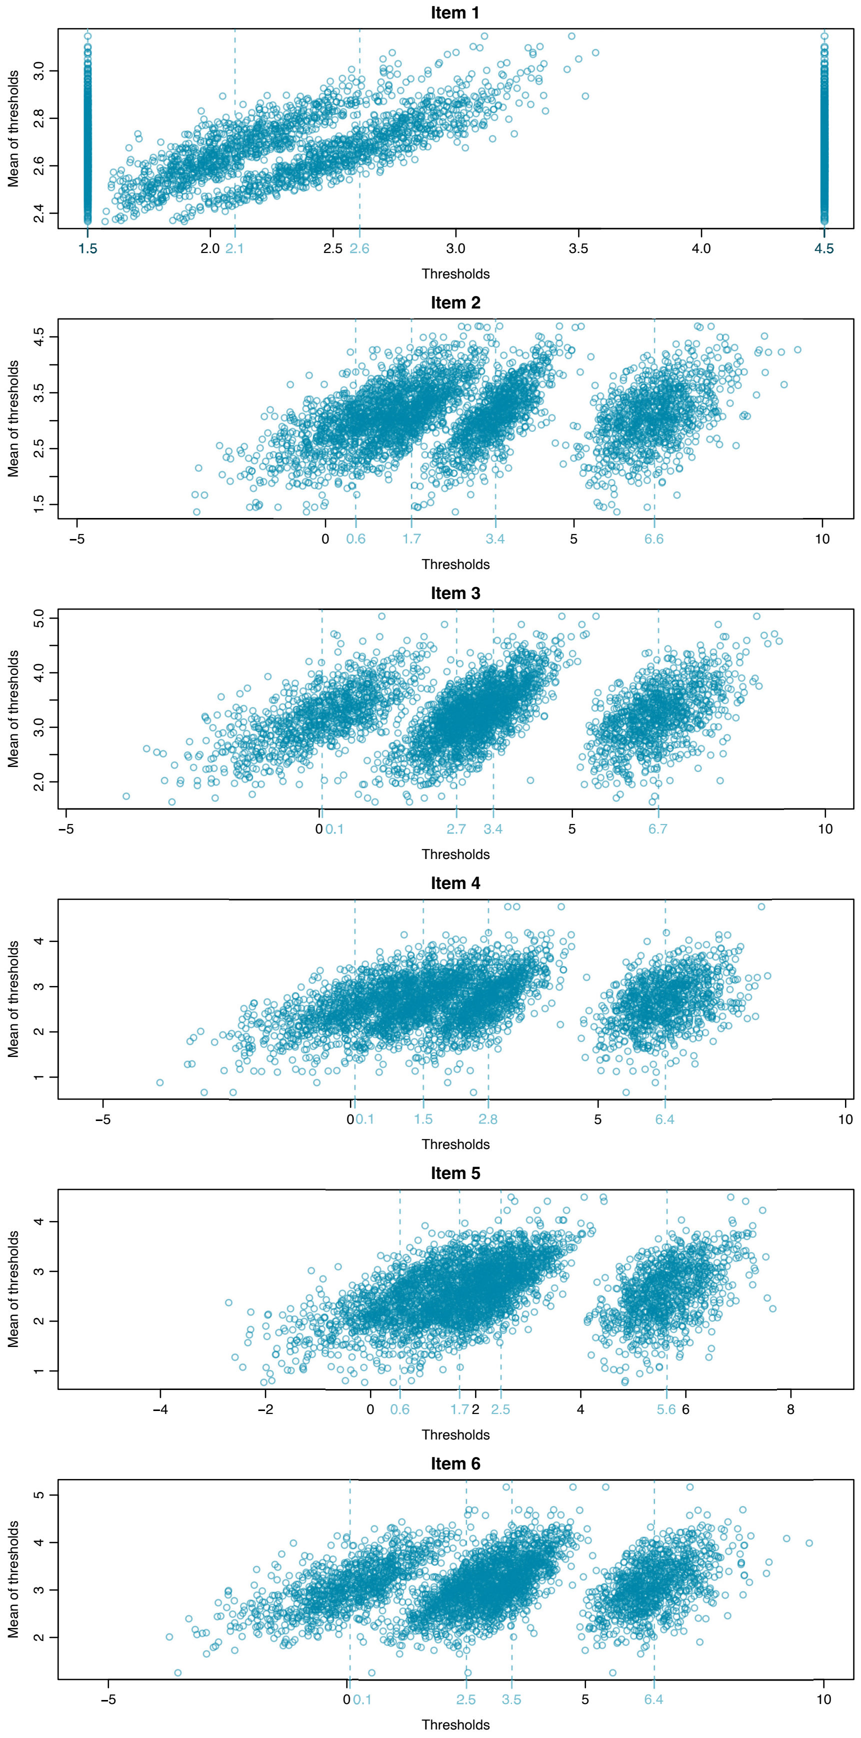


**Fig. 6** Posterior distributions of each item thresholds of the Likert scale for the acceptance of the virtual agents. Dashed lines indicate the means of the thresholds estimations.

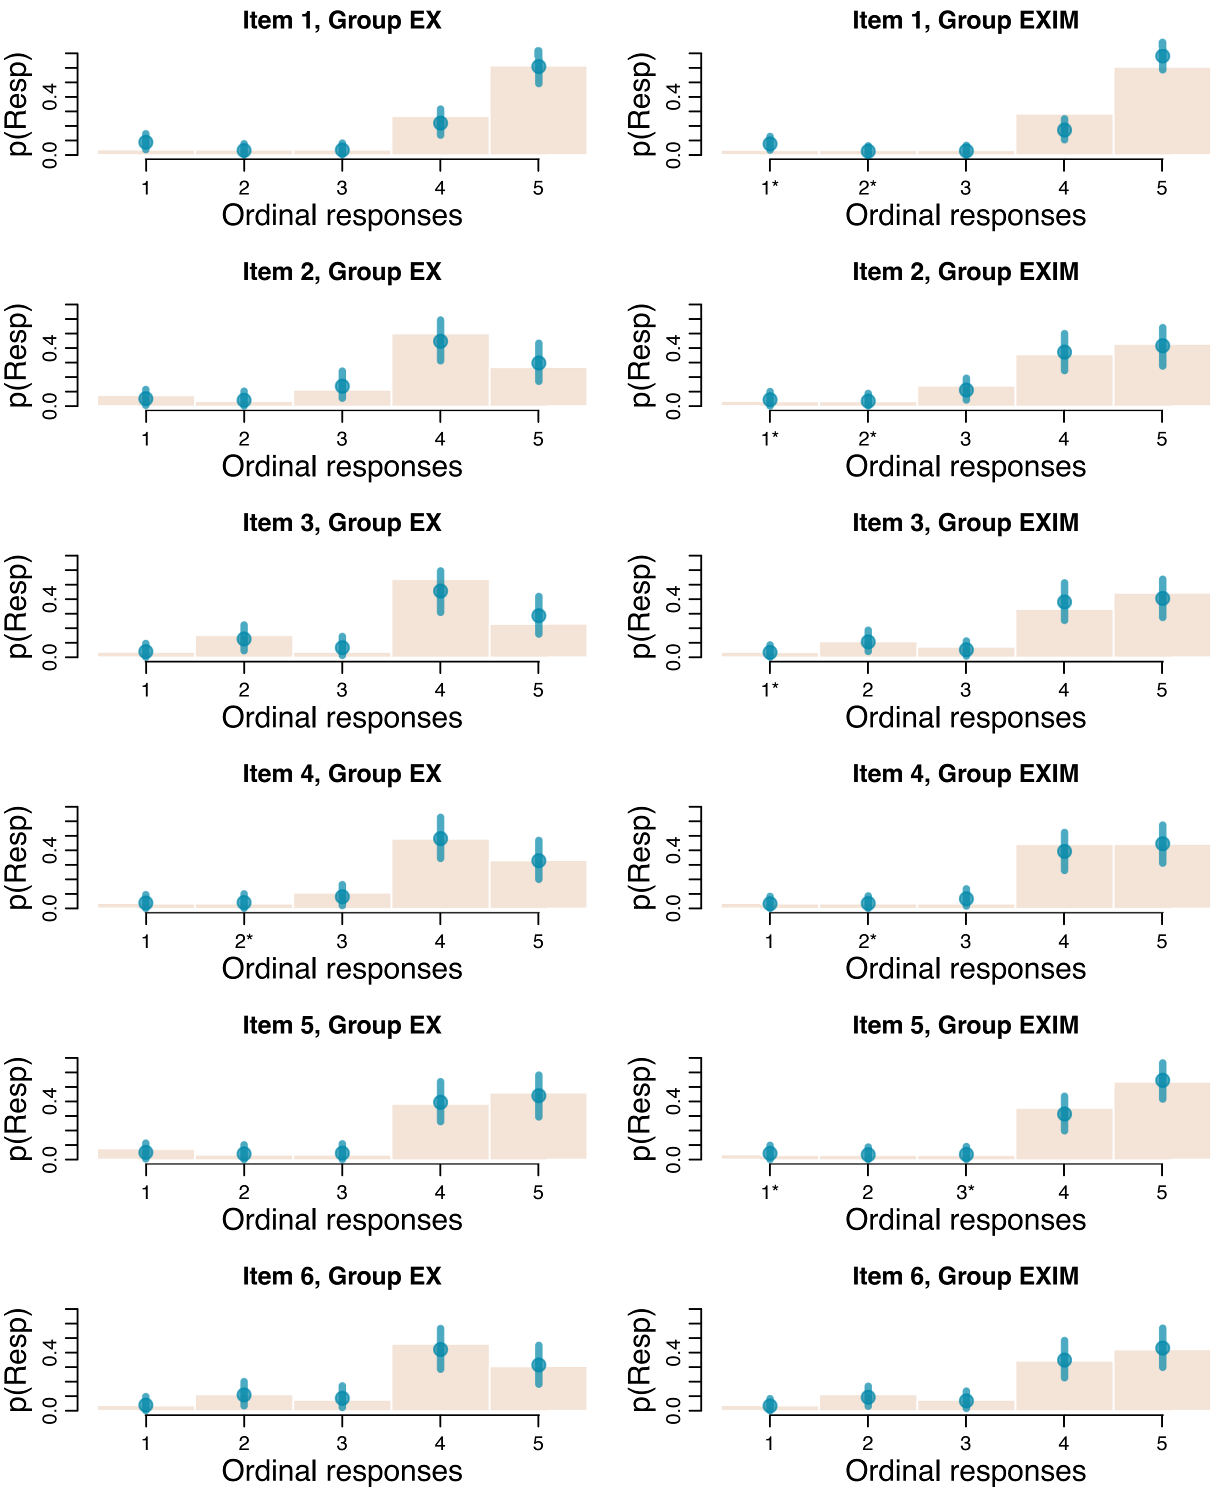


**Fig. 7** Acceptance data histograms superimposed with estimated probabilities to check model adequacy. Each blue dot indicates the estimated median and the vertical line represents the 95% HDI. Levels that had extra answers added are marked with an asterisk (*).

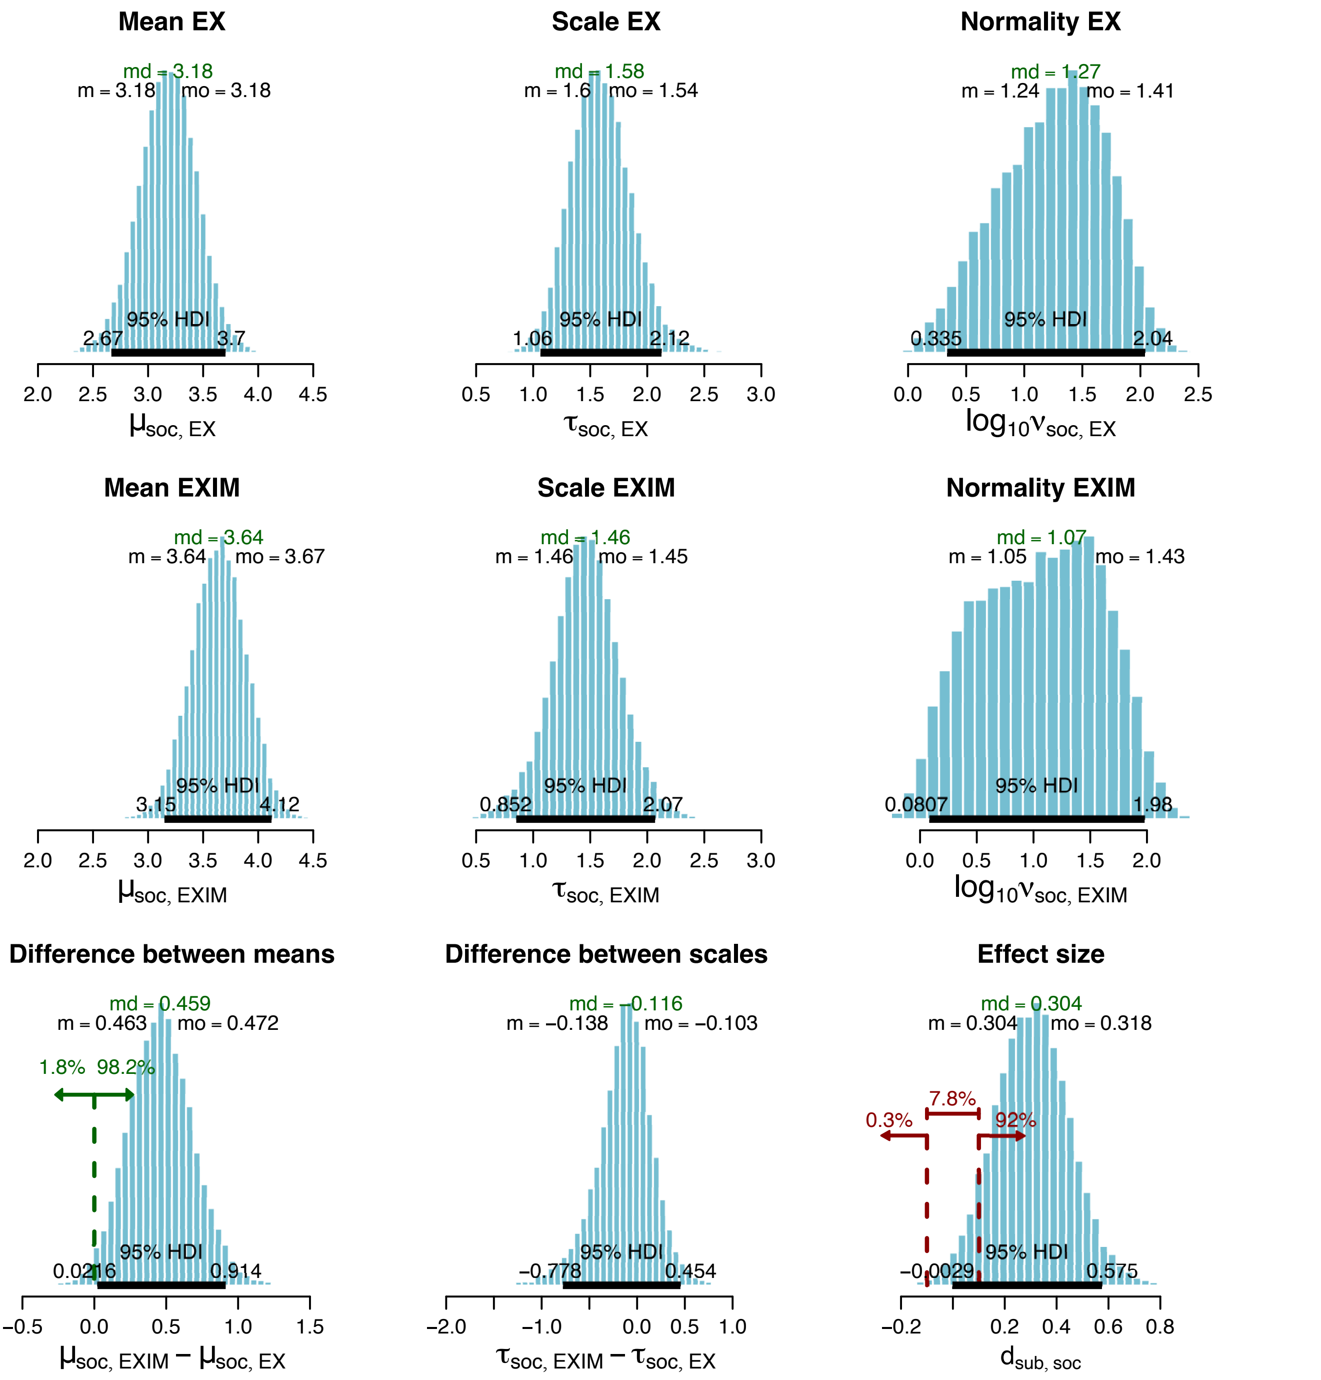


**Fig. 8** Results of the Bayesian inference of the sociability of the virtual agents in EX and EXIM configurations. The first two rows show the posterior distributions of the mean $\mu$, scale $\tau$, and normality $\nu$ (in log scale) of the latent $t$ distribution of each group. On the left and center of the last row are the distributions of difference between the means and scales of the two groups, and on the right, the distribution of the effect size $d_{\text{sub}}$. Mean $(m)$, median $(md)$, mode $(mo)$, and the limits of the 95% HDI are annotated in the distributions. Dashed vertical lines indicate the null value $(\mu_{\text{EXIM}} - \mu_{\text{EX}} = 0)$ in the distribution of the difference between means and the ROPE in the effect size distribution together with the percentages of the distribution below, between and above the values associated with the ROPE and the null value.

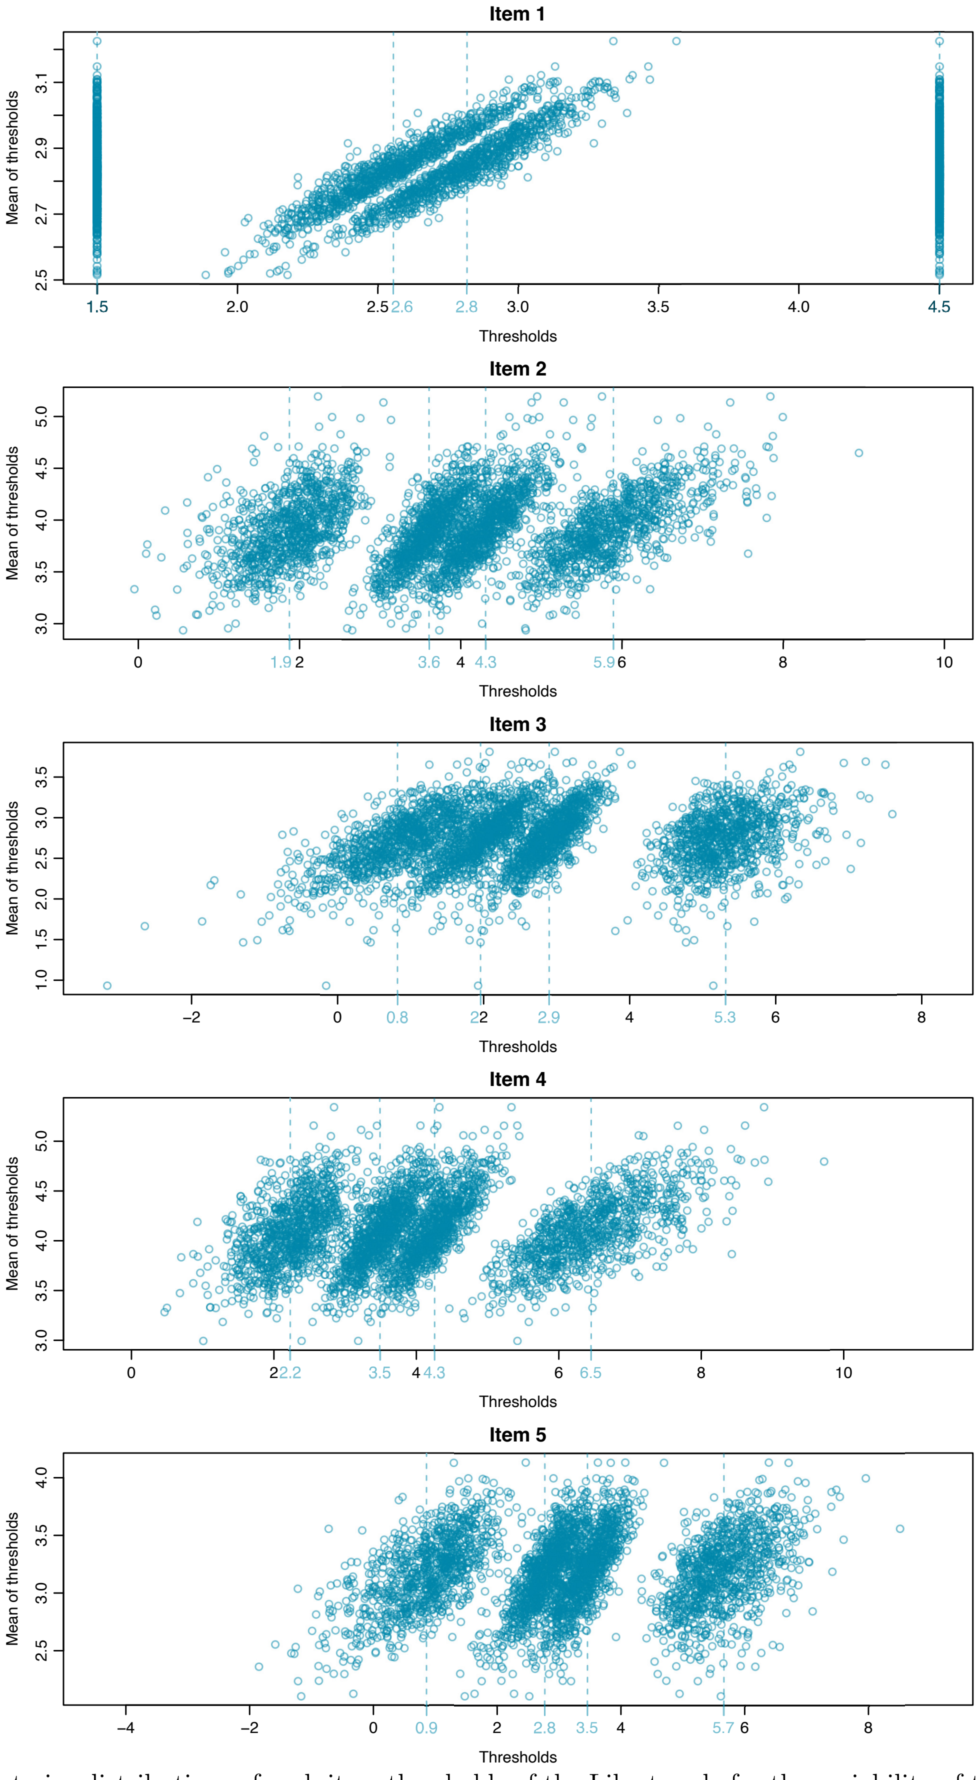


**Fig. 9** Posterior distributions of each item thresholds of the Likert scale for the sociability of the virtual agents. Dashed lines indicate the means of the thresholds estimations.

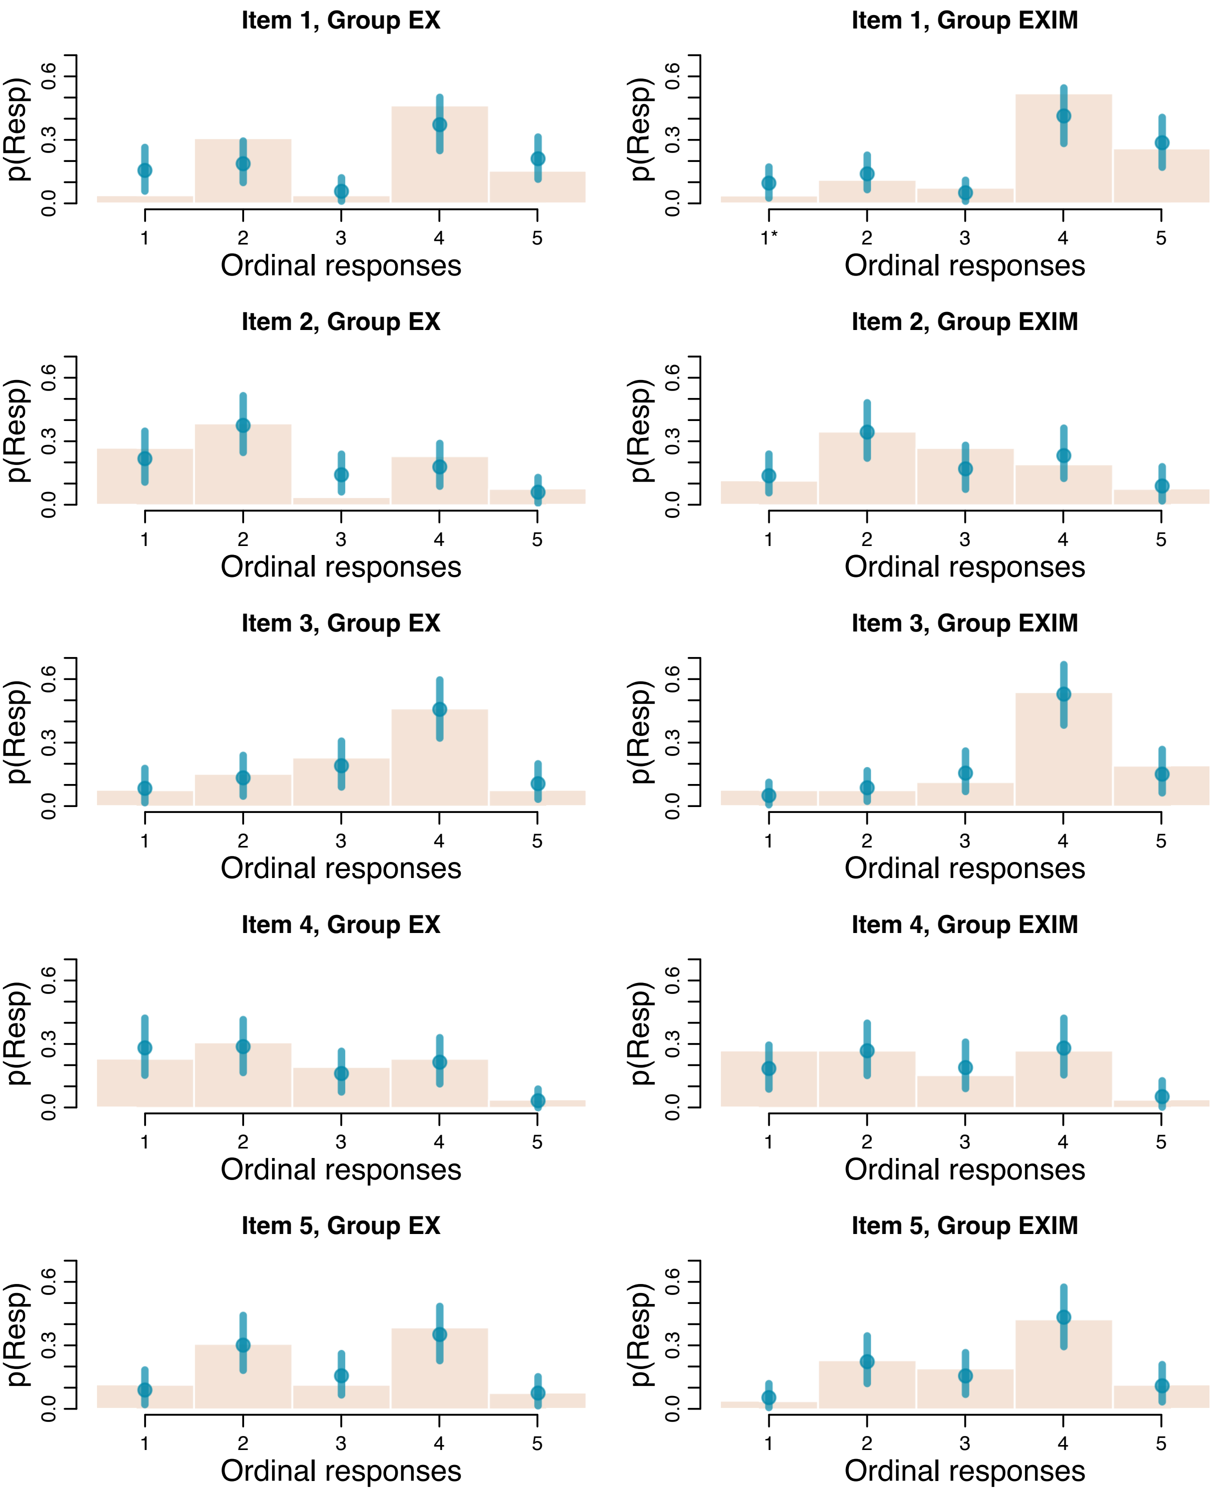


**Fig. 10** Sociability data histograms superimposed to estimated probabilities to check model adequacy. Each blue dot indicates the estimated median and the vertical line the 95% HDI. Levels that had extra answers added are marked with an asterisk (*).

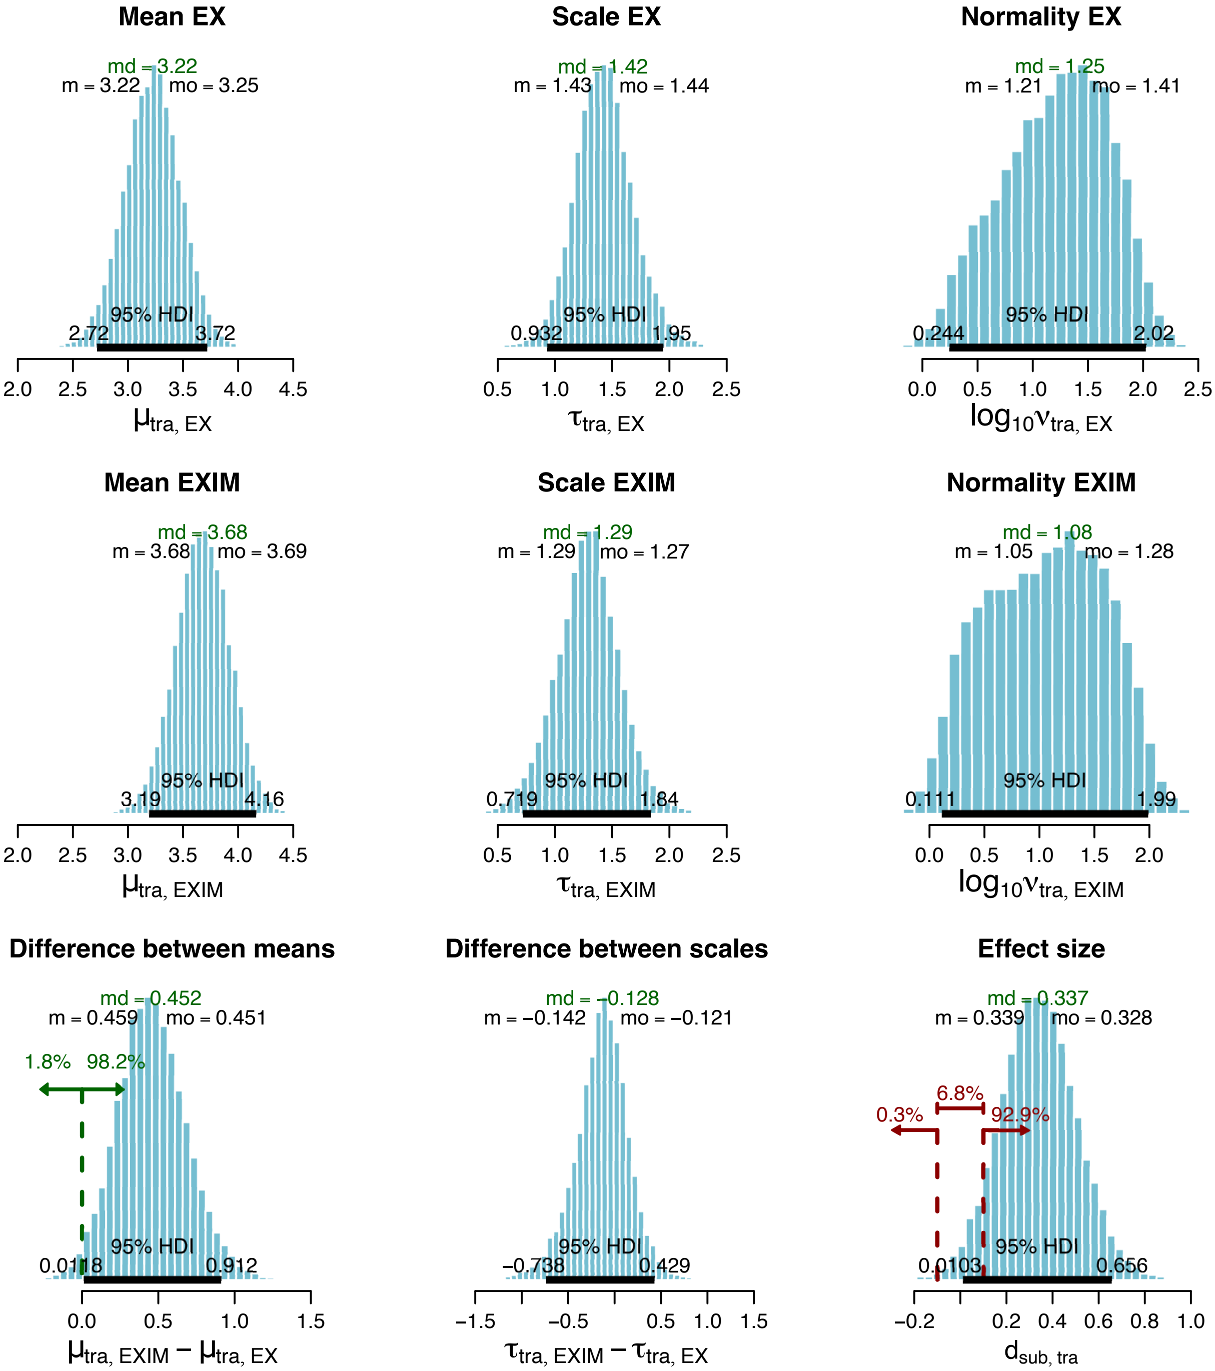


**Fig. 11** Results of the Bayesian inference of the transparency of the virtual agents in EX and EXIM configurations. The first two rows show the posterior distributions of the mean $\mu$, scale $\tau$, and normality $\nu$ (in log scale) of the latent $t$ distribution of each group. On the left and center of the last row are the distributions of difference between the means and scales of the two groups, and on the right, the distribution of the effect size $d_{\text{sub}}$. Mean $(m)$, median $(md)$, mode $(mo)$, and the limits of the 95% HDI are annotated in the distributions. Dashed vertical lines indicate the null value $(\mu_{\text{EXIM}} - \mu_{\text{EX}} = 0)$ in the distribution of the difference between means and the ROPE in the effect size distribution together with the percentages of the distribution below, between and above the values associated with the ROPE and the null value.

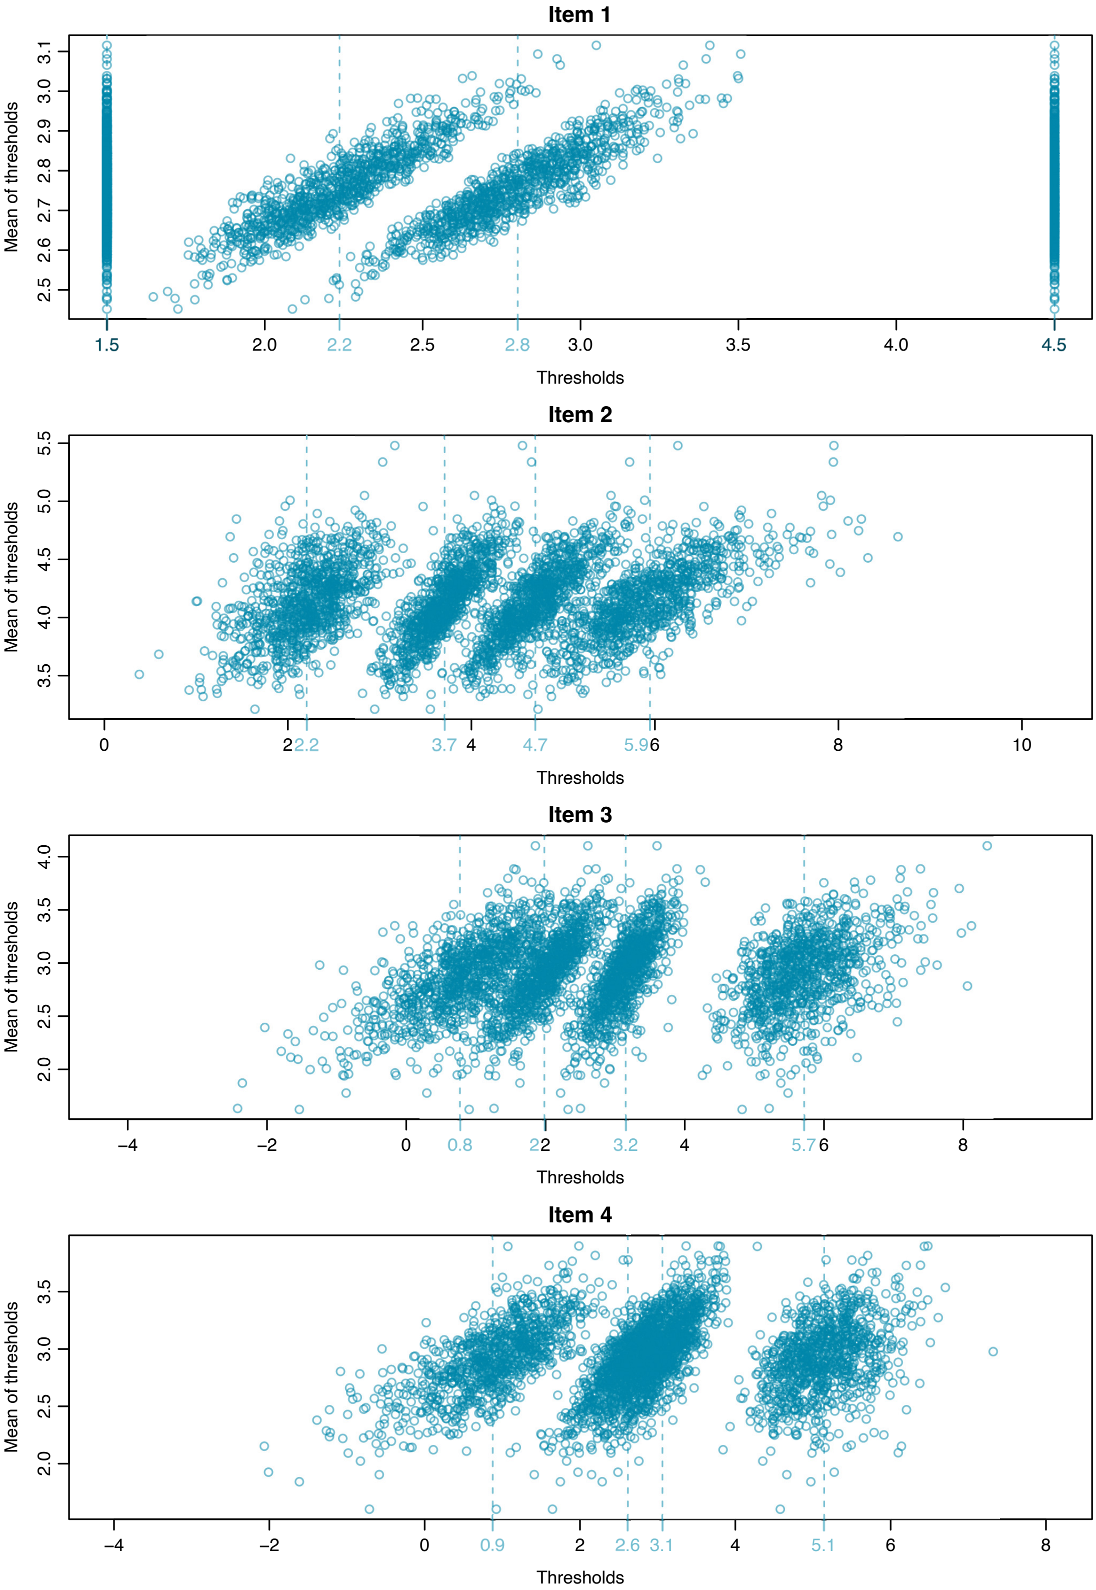


**Fig. 12** Posterior distributions of each item thresholds of the Likert scale for the transparency of the virtual agents. Dashed lines indicate the means of the thresholds estimations.

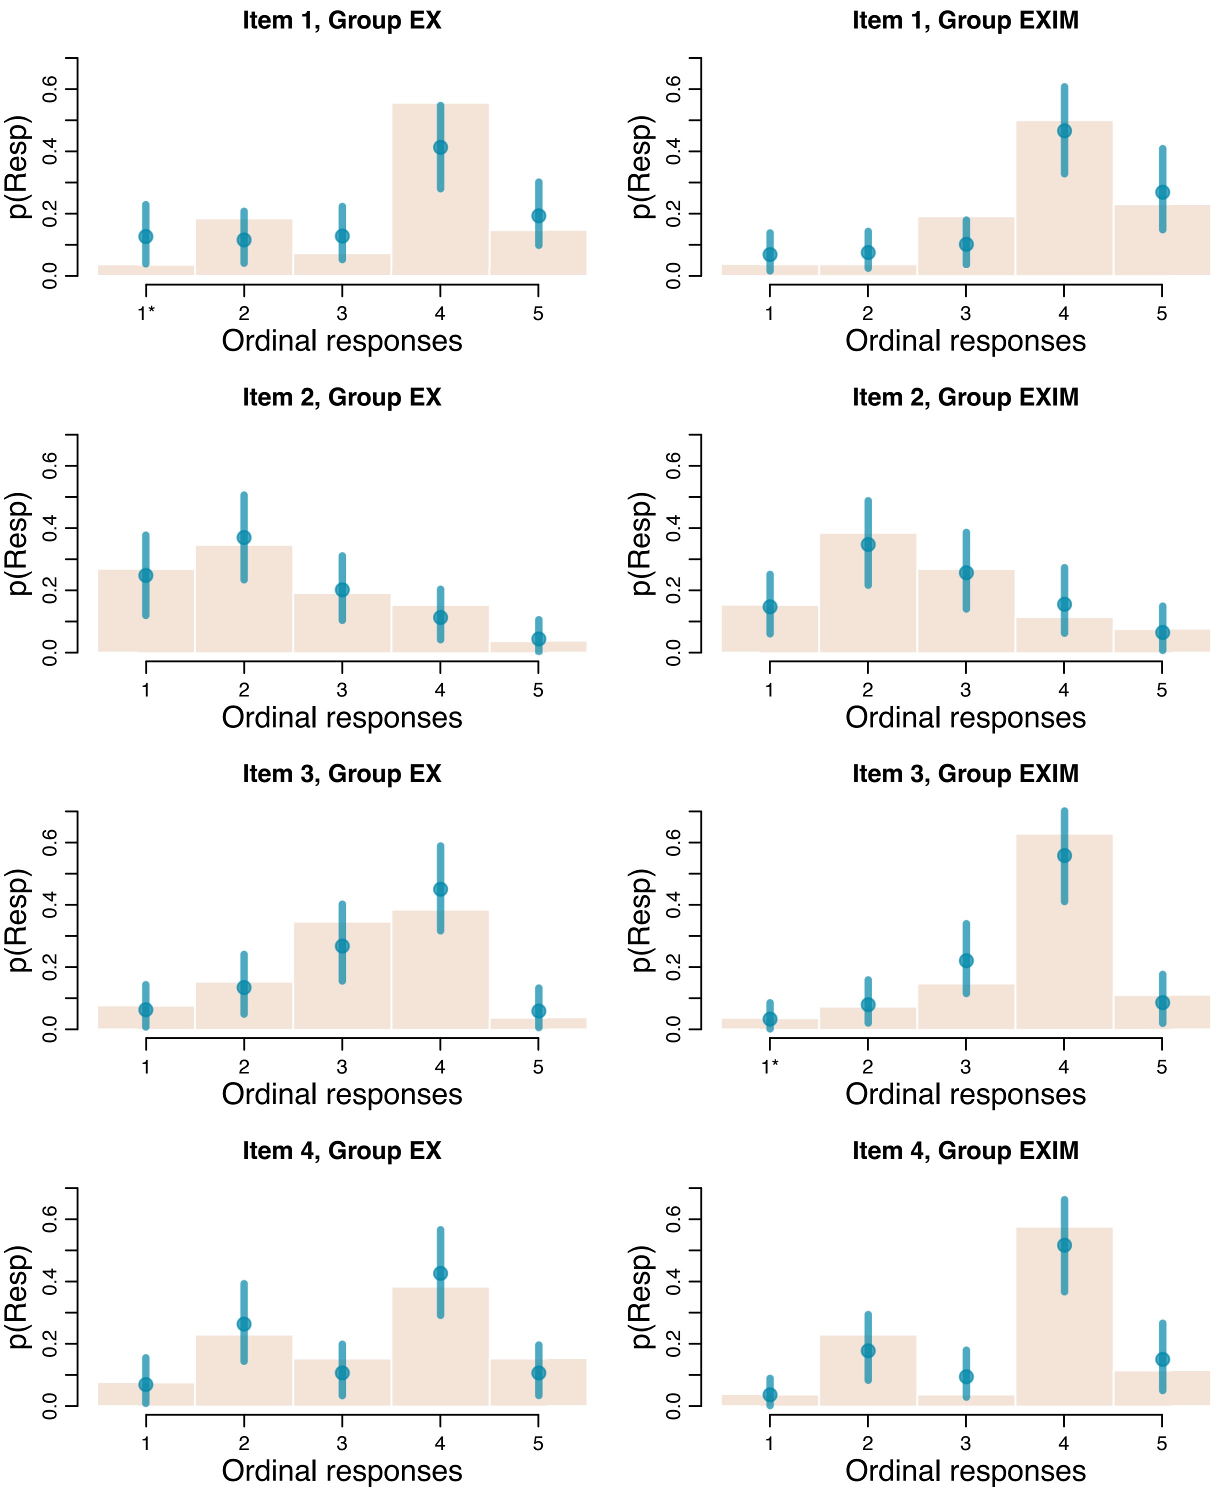


**Fig. 13** Transparency data histograms superimposed to estimated probabilities to check model adequacy. Each blue dot indicates the estimated median and the vertical line the 95% HDI. Levels that had extra answers added are marked with an asterisk (*).

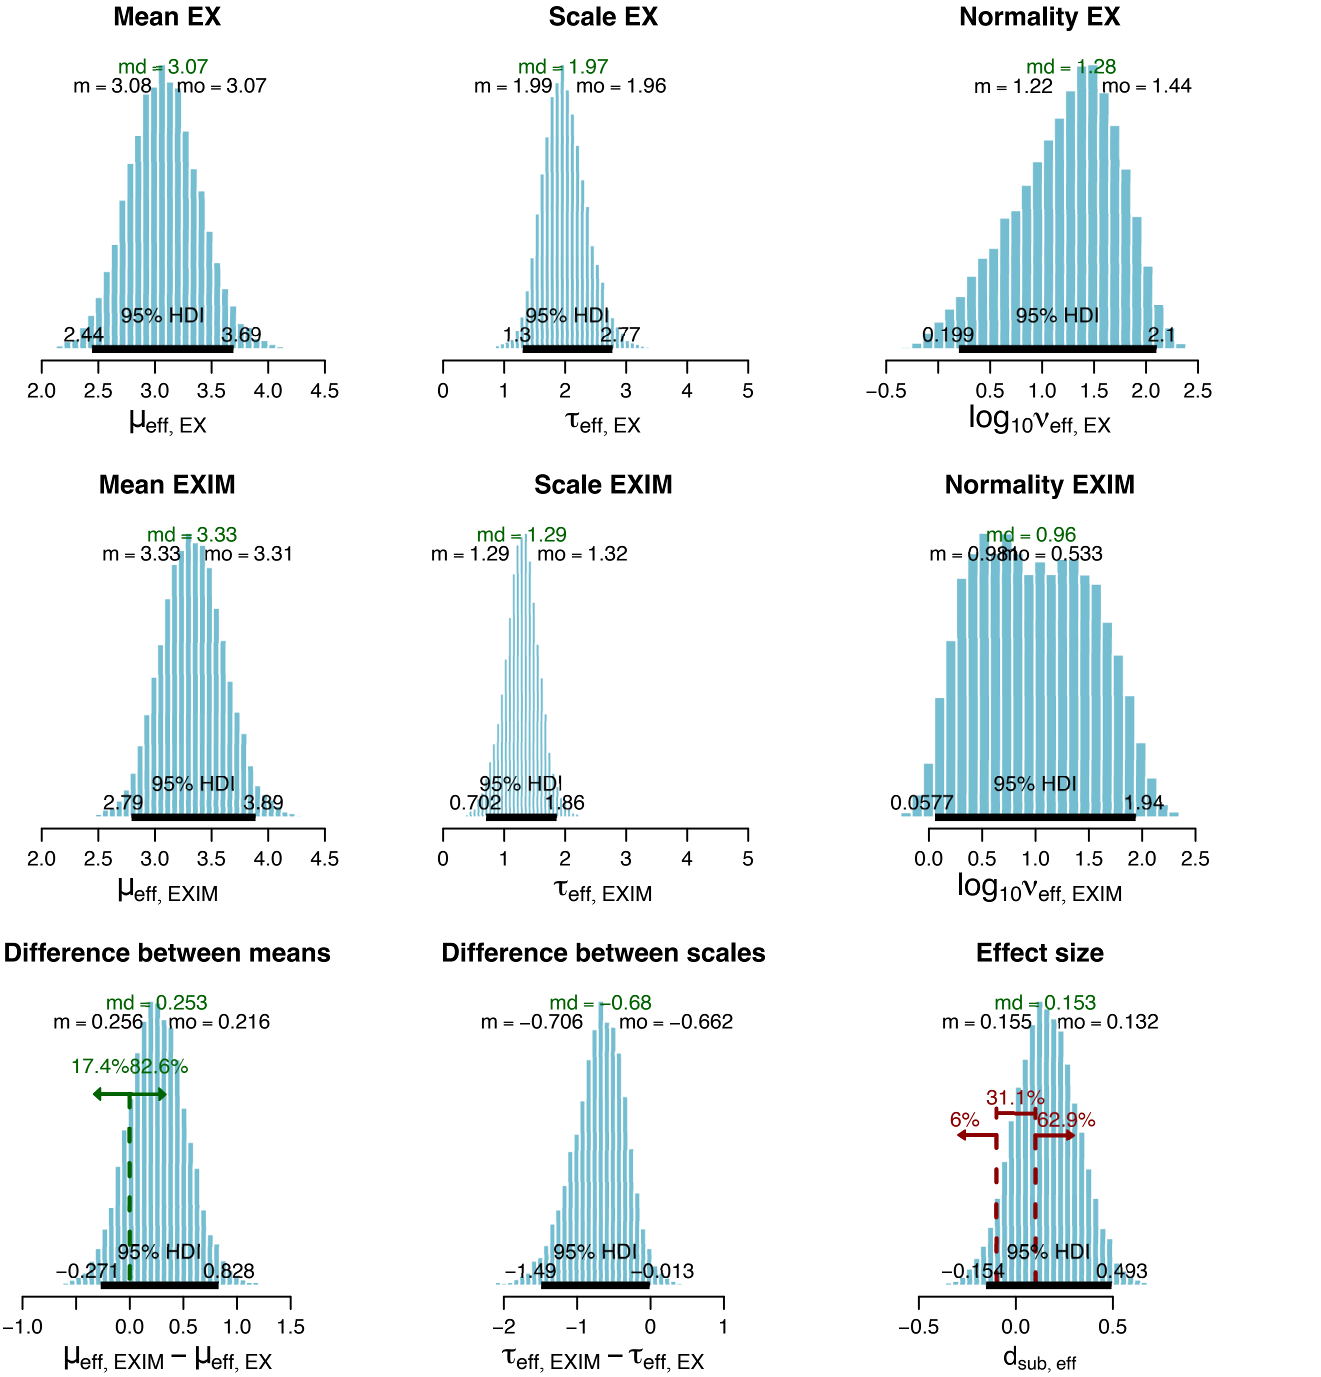


**Fig. 14** Results of the Bayesian inference of the perceived efficiency of the interactions in EX and EXIM configurations. The first two rows show the posterior distributions of the mean $\mu$, scale $\tau$, and normality $\nu$ (in log scale) of the latent $t$ distribution of each group. On the left and center of the last row are the distributions of difference between the means and scales of the two groups, and on the right, the distribution of the effect size $d_{\text{sub}}$. Mean $(m)$, median $(md)$, mode $(mo)$, and the limits of the 95% HDI are annotated in the distributions. Dashed vertical lines indicate the null value $(\mu_{\text{EXIM}} - \mu_{\text{EX}} = 0)$ in the distribution of the difference between means and the ROPE in the effect size distribution together with the percentages of the distribution below, between and above the values associated with the ROPE and the null value.

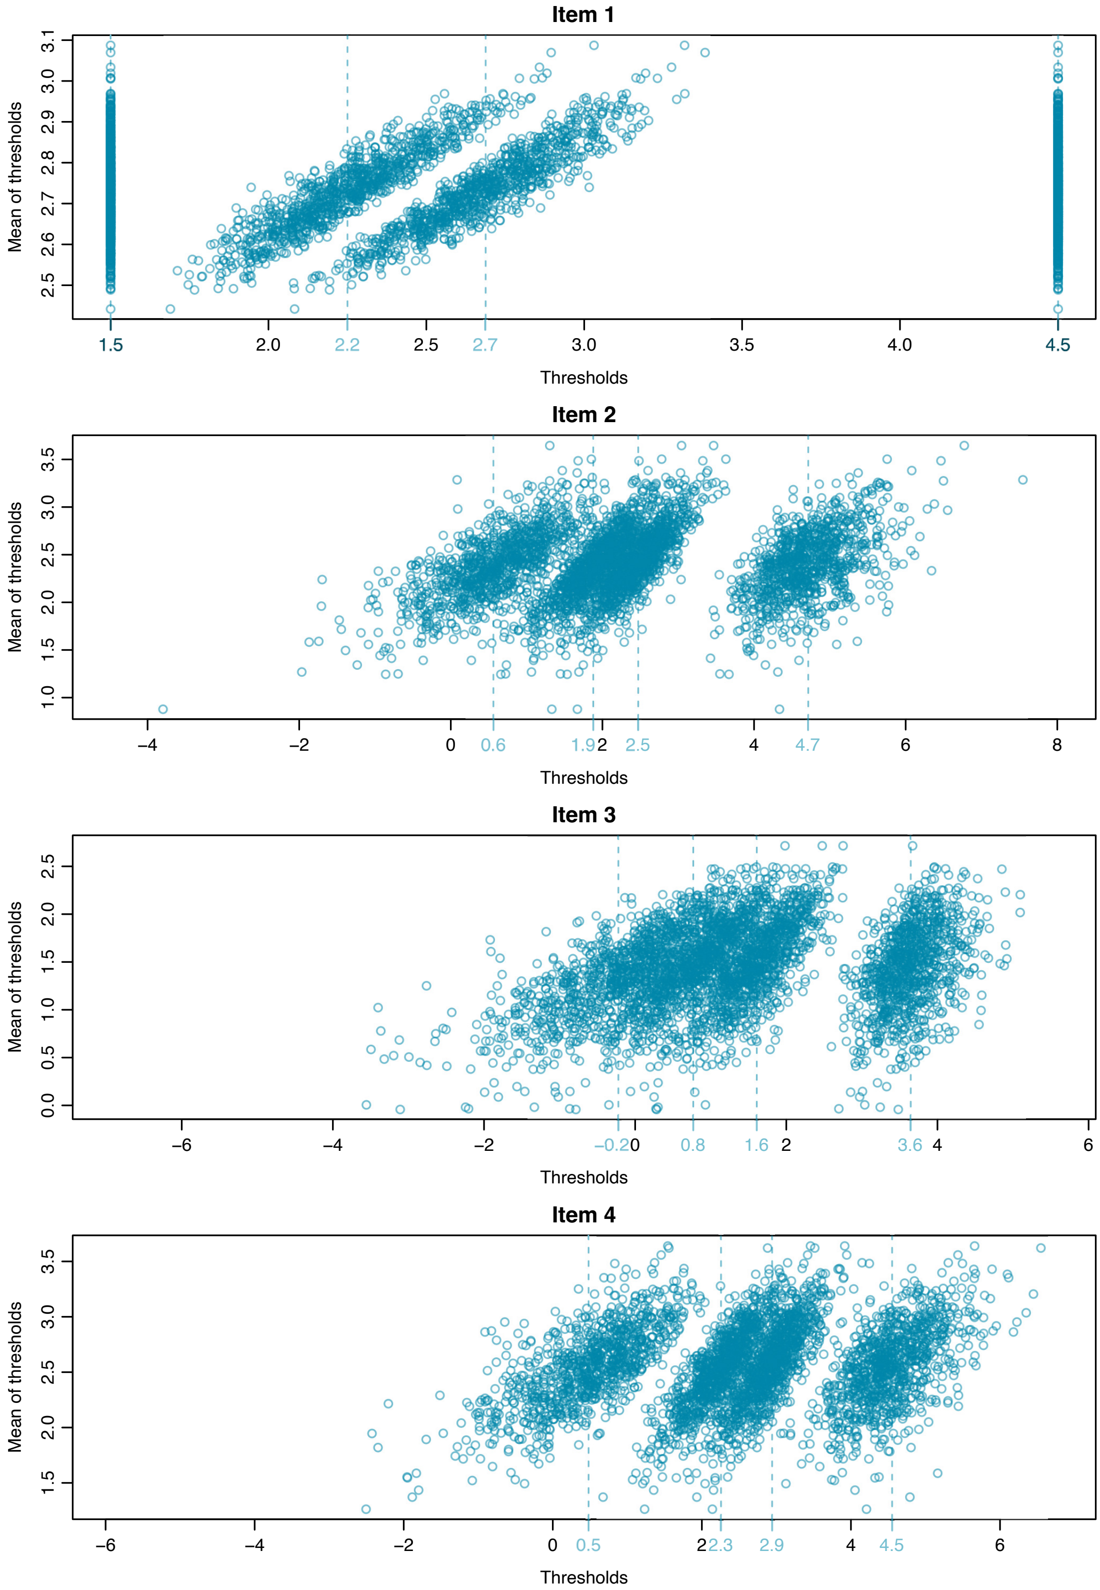


**Fig. 15** Posterior distributions of each item thresholds of the Likert scale for the perceived efficiency of the interactions. Dashed lines indicate the means of the thresholds estimations.

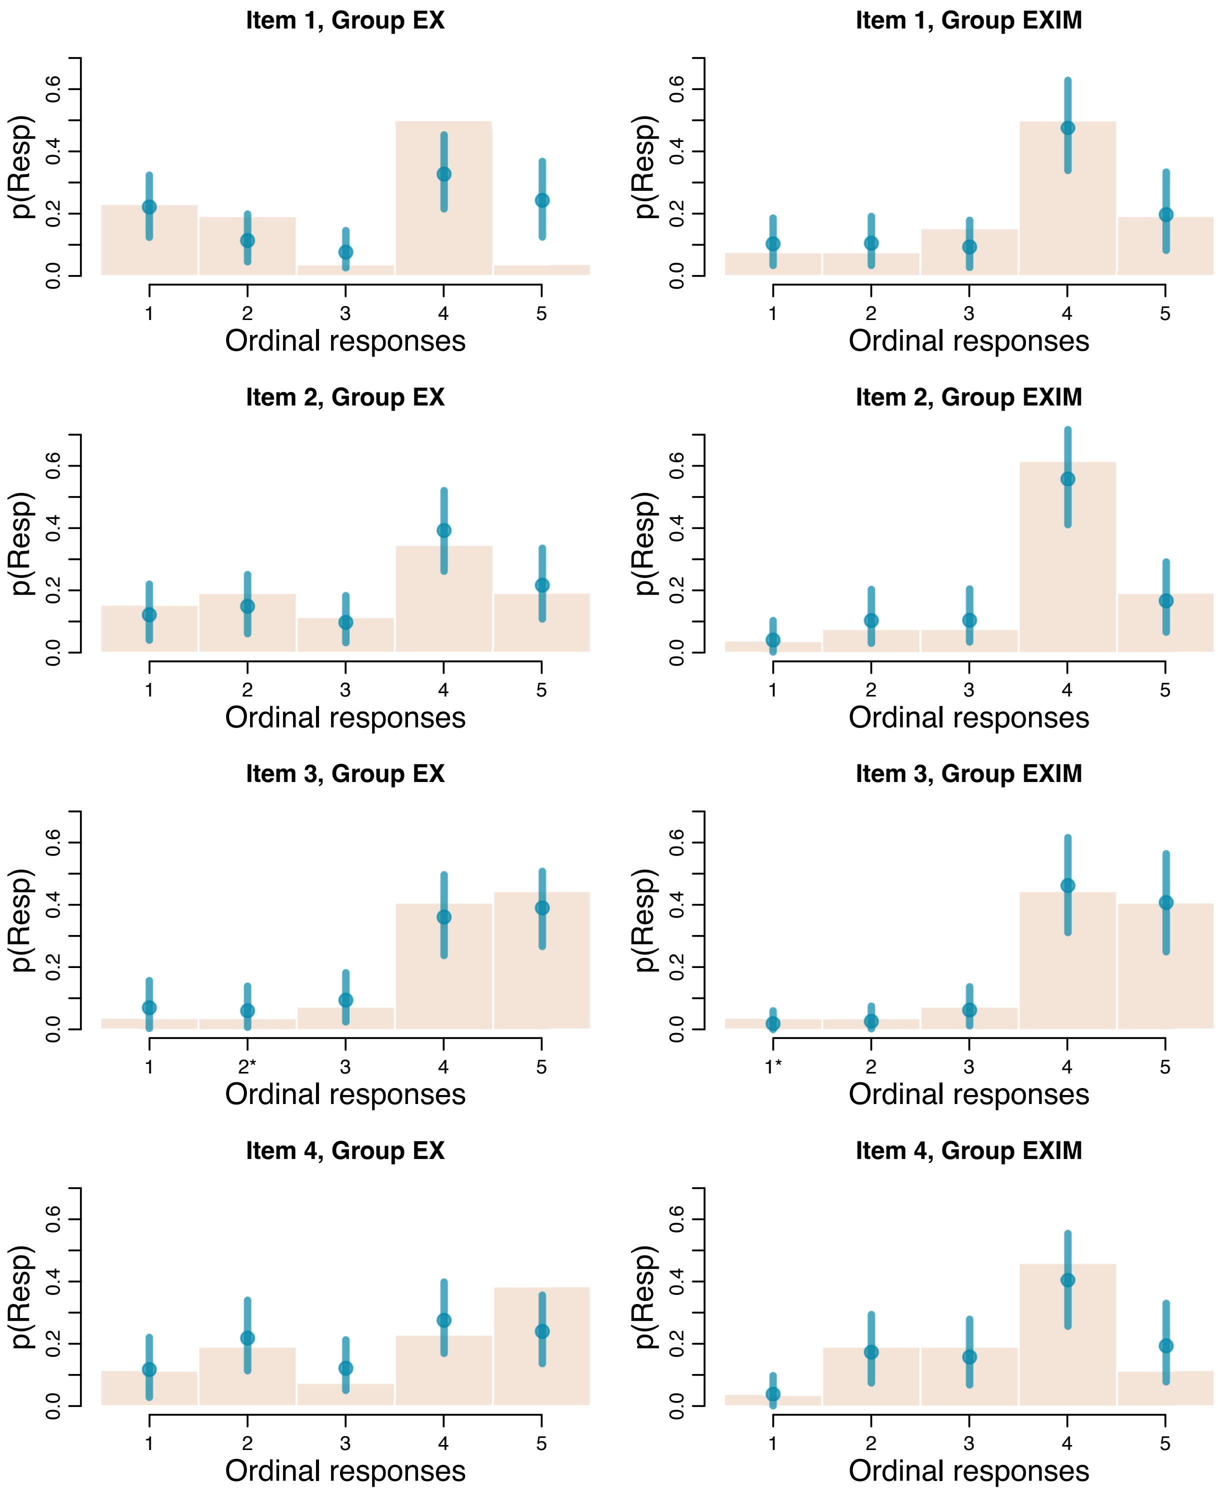


**Fig. 16** Perceived efficiency data histograms superimposed to estimated probabilities to check model adequacy. Each blue dot indicates the estimated median and the vertical line the 95% HDI. Levels that had extra answers added are marked with an asterisk (*).
